# Supplementary material for: Non-compact groups, tensor operators and applications to quantum gravity
Source: arXiv:1609.07795 source file (2016-09-25)
Supplement: Supplementary file 1 [file group_representations.tex]

\chapter{Group representations of \texorpdfstring{Spin(2,1)}{\Spin(2,1)} and \texorpdfstring{Spin(3,1)}{\Spin(3,1)}}
\label{app:group_representations}

\section{Group representations of \texorpdfstring{Spin(2,1)}{\Spin(2,1)}}
\label{app:group_representations_3d}

\subsection*{Positive discrete series}
\begin{equation}
\begin{pmatrix}
\alpha & \beta\\
\conj\beta & \conj\alpha
\end{pmatrix}
f(z)=
(\conj\alpha-\beta z)^{-2j-2} \,f \paren*{\frac{\alpha z - \conj\beta}{\conj\alpha-\beta z}}
\end{equation}

\begin{equation}
\braket{f,g}:=
\begin{dcases}
\int_{\abs{z}<1}\conj{f(z)}g(z)\paren*{1-\abs{z}^2}^{2j}\,\eder z & \casesif j\geq 0
\\
\sup_{0\leq\rho<1}\int_{0}^{2\pi} \conj{f(\rho e^{\ii\theta})}g(\rho e^{\ii\theta})\,\eder\theta & \casesif j=-\half
\end{dcases}
\end{equation}

\begin{subequations}
\begin{align}
J_0 f(z) &= z\pder{f}{z}+(j+1)f(z)\\
J_+ f(z) &= \ii z^2\pder{f}{z}+2 \ii (j+1) z f(z)\\
J_- f(z) &= -\ii \pder{f}{z}
\end{align}
\end{subequations}

\begin{equation}
\ket{j,m}=f_{j,m}(z):=\mathcal{N}_{j,m}\,z^{m-j-1},\quad m \in \set{j+1,j+2,\dotsc}
\end{equation}

\begin{equation}
\mathcal{N}_{j,m}=(-\ii)^m
\begin{cases}
\pi^{-\shalf}\sqrt{\frac{(j+m)!}{(2j)!(m-j-1)!}} &\casesif j\geq 0\\
(2\pi)^{-\shalf} &\casesif j=-\half
\end{cases}
\end{equation}

\subsection*{Negative discrete series}
\begin{equation}
\begin{pmatrix}
\alpha & \beta\\
\conj\beta & \conj\alpha
\end{pmatrix}
f(\conj z)=
(\alpha-\conj\beta \conj z)^{-2j-2} \,f \paren*{\frac{\conj\alpha \conj z - \beta}{\alpha-\conj\beta \conj z}}
\end{equation}

\begin{equation}
\braket{f,g}:=
\begin{dcases}
\int_{\abs{z}<1}\conj{f(\conj z)}g(\conj z)\paren*{1-\abs{z}^2}^{2j}\,\eder z & \casesif j\geq 0
\\
\sup_{0\leq\rho<1}\int_{0}^{2\pi} \conj{f(\rho e^{-\ii\theta})}g(\rho e^{-\ii\theta})\,\eder\theta & \casesif j=-\half
\end{dcases}
\end{equation}

\begin{subequations}
\begin{align}
J_0 f(\conj z) &= -\conj z\pder{f}{\conj z}  -(j+1)f(\conj z)\\
J_+ f(\conj z) &= -\ii \pder{f}{\conj z}\\
J_- f(\conj z) &= \ii \conj z^2\pder{f}{\conj z}+2 \ii (j+1) \conj z f(\conj z)
\end{align}
\end{subequations}

\begin{equation}
\ket{j,m}=f_{j,m}(\conj z):=\mathcal{N}_{j,m}\,{\conj z}^{-m-j-1},\quad m \in \set{-j-1,-j-2,\dotsc}
\end{equation}

\begin{equation}
\mathcal{N}_{j,m}=(-\ii)^m
\begin{cases}
\pi^{-\shalf}\sqrt{\frac{(j+m)!}{(2j)!(m-j-1)!}} &\casesif j\geq 0\\
(2\pi)^{-\shalf} &\casesif j=-\half
\end{cases}
\end{equation}

\subsection*{Continuous series}

\begin{equation}
\begin{pmatrix}
\alpha & \beta\\
\conj\beta & \conj\alpha
\end{pmatrix}
f(e^{\ii\theta})=
\abs*{\conj\alpha-\beta e^{\ii\theta}}^{-2(j+1+\varepsilon)} \paren*{\conj\alpha-\beta e^{\ii\theta}}^{2\varepsilon}\,f \paren*{\frac{\alpha e^{\ii\theta} - \conj\beta}{\conj\alpha-\beta e^{\ii\theta}}}
\end{equation}

\begin{equation}
\braket{f,g}:=\frac{1}{2\pi}\int_{0}^{2\pi}\conj{f(e^{\ii\theta})}g(e^{\ii\theta})\,\eder\theta
\end{equation}

\begin{subequations}
\begin{align}
J_0 f(e^{\ii\theta}) &= -\ii\pder{f}{\theta} - \varepsilon f(e^{\ii\theta})\\
J_+ f(e^{\ii\theta}) &= e^{\ii\theta} \paren*{\pder{f}{\theta}+ \ii\paren{j+1-\varepsilon} f(e^{\ii\theta})}\\
J_- f(e^{\ii\theta}) &= e^{-\ii\theta} \paren*{-\pder{f}{\theta}+ \ii\paren{j+1+\varepsilon} f(e^{\ii\theta})}
\end{align}
\end{subequations}

\begin{equation}
\ket{j,m}=f_{j,m}(e^{\ii\theta})=\mathcal{N}_{j,m}\,e^{\ii(m+\varepsilon)\theta}
\end{equation}

\begin{equation}
\mathcal{N}_{j,m}:=\prod_{k=1}^{\abs{m}}\frac{\sqrt{j+k}}{\sqrt{j-k+1}}
\end{equation}

\section{Group representations of \texorpdfstring{Spin(3,1)}{\Spin(3,1)}}
\label{app:group_representations_4d}
